# Supplementary material for: Robust and Effective Malware Detection through Quantitative Data Flow Graph Metrics
Source: arXiv:1502.01609 source file (2015-02-12)
Supplement: Supplementary file 1 [file appendix.tex]

\todo{add stuff like further evaluation material here if needed}
